# Supplementary material for: Optimization of the Model Predictive Control Meta-Parameters Through Reinforcement Learning
Source: arXiv:2111.04146 source file (2021-11-07)
Supplement: Supplementary file 1 [file appendixC.tex]

\section{Background}
\subsection{Value Function Estimation}
A value function measures the expected total sum of costs accrued from being in any given state and from there always acting according to a given control law $\pi$, until the end of the episode (or in an infinite horizon in the non-episodic case) \eqref{eq:valfn}. The ideal choice for the terminal cost $m(x_{N_t})$ of the \gls{mpc} scheme would be the optimal value function \eqref{eq:vstar} which is the value function corresponding to the optimal control law ${\pi^*}$ that delivers the optimal control input at every step. Equation \eqref{eq:vstar} is written as a recursive relationship in $V^{\pi^*}$ called the Bellman equation, where the value of a given state is decomposed into the one-step optimal cost and the total value from the subsequent state. Computing $V^{\pi^*}$ exactly from this equation is however intractable for problems with continuous state and/or input spaces, and iterative approaches such as Q-learning requires a prohibitively large amount of data.

\begin{align}
    V^\pi(x_t, \hat{p}_t) &= \mathbb{E}\left[\sum_{t'=t}^T \rho^{t'} \ell(x_{t'}, \pi(x_{t'}, \hat{p}_{t'}), \hat{p}_{t'}) \right] \label{eq:valfn} \\
    V^{\pi^*}(x_t, \hat{p}_t) &= \min_u \ell(x_t, u_t, \hat{p}_t) + \rho V^{\pi^*}(x_{t+1}, \hat{p}_{t+1}), \enspace \forall \> t, x, \hat{p} \label{eq:vstar}
\end{align}

The control paradigm of \gls{mpc} is however centered around providing local approximations to $\pi^*$, and as such, the \gls{mpc}'s value function $V^{\pi^{\mathrm{MPC}}}$ is a good surrogate for the optimal value function $V^{\pi^{*}}$. This value function is not necessarily directly computable either, as it would require running the \gls{mpc} with an infinite prediction horizon (or at least equal to the remaining steps of the episode). However, it can be approximated using fitted value iteration on data gathered by running $\pi^{\mathrm{MPC}}$ on the system to be optimized. We label the approximated \gls{mpc} value function $\hat{V}^{\pi^{\mathrm{MPC}}}_{\theta^{V}}$, where $\theta^{V}$ are the parameters of the value function approximator. These parameters are iteratively updated to minimize the \gls{msbe}:

\begin{align}
        \theta^{V} &\leftarrow \argmin_{\theta^{V}} \mathbb{E} \left[ \left(y(x, \hat{p}) - \hat{V}_{\theta^{V}} (x, \hat{p})\right)^2\right] \label{eq:val_fn_update} \\
        y(x_t, \hat{p}_t) &=  \mathbb{E}\left[\ell(x_t, \pi^{\textrm{MPC}}(x_t, \hat{p}_t, N_t), \hat{p}_t) + \rho \hat{V}_{\theta^V}(x_{t+1}, \hat{p}_{t+1})\right] \label{eq:val_fn_update:target}
\end{align}

Here, \eqref{eq:val_fn_update:target} is called the regression target and corresponds to the condition on the value function imposed by the one-step Bellman equation \eqref{eq:vstar}. Since the \gls{mpc} scheme delivers $N_t$-step approximations to the optimal control law $\pi^{*}$, one can modify the update rule to instead regress onto the N-step target \cite{lowrey2018plan}:

\begin{equation}
        y(x_t, \hat{p}_t) = \mathbb{E}\left[\sum_{k=0}^{N-1}\rho^k\ell(x_k, u_k, \hat{p}_k) + \rho^N \hat{V}_{\theta^V}(x_N, \hat{p}_N)\right] \label{eq:nstep}
\end{equation}

With this regression target a larger share of the value of the future trajectory from $x_t$ is known exactly (through the observed costs $\ell$) and the contribution of the estimated bootstrapping component $\hat{V}_{\theta^V}(x_N, \hat{p}_N)$ is reduced by a factor of $\rho^N$. This typically leads to accelerated convergence and higher stability in the learning process \citep{vanseijen2016effective,sutton_reinforcement_2018}.

\subsection{Linear Quadratic Regulator}
The \gls{lqr} \citep{bertsekas1995dynamic} is a state-feedback controller that arises as the optimal solution to unconstrained control problems where the dynamics are linear, and the reward is quadratic. In this paper we focus on the discrete-time formulation of the \gls{lqr}. In the infinite-horizon case, the control law \eqref{eq:lqr:control_law} consists of a feedback gain matrix, $\matr{K_\infty}$ \eqref{eq:lqr:K}, that is derived from the dynamics matrices $\matr{A}$ and $\matr{B}$, the reward weighting matrices $\matr{Q}$, $\matr{R}$ and $\matr{N}$, and the solution $\matr{S_\infty}$ to the \gls{dare} \eqref{eq:lqr:dare} parameterized by $\matr{A}, \matr{B}, \matr{Q}, \matr{R}, \matr{N}$. In this paper we consider $\theta^\mathrm{L} = \left[\matr{Q}, \matr{R}, \matr{N}\right]^\top$ as parameters of the \gls{lqr} controller that can be optimized:
\begin{align}
    0 &= \matr{A}^\top \matr{S} \matr{A} - \matr{S} - (\matr{A}^\top \matr{S} \matr{B} + \matr{N})(\matr{B}^\top \matr{S} \matr{B} + \matr{R})^{-1} (\matr{B}^\top \matr{S} \matr{A} + \matr{N}^\top) + \matr{Q} \label{eq:lqr:dare} \\
    \matr{K} &= (\matr{B}^\top \matr{S} \matr{B} + \matr{R})^{-1}(\matr{B}^\top \matr{S} \matr{A} + \matr{N}^\top) \label{eq:lqr:K} \\
    u^\mathrm{L}_k(x_k) &= \pi^{\mathrm{L}}_{\theta^{\mathrm{L}}}(x_k) = -\matr{K} x_k \label{eq:lqr:control_law}
\end{align}

The \gls{lqr} control problem we consider is formally stated as:

\begin{align}
    \min_{x, u} \quad &\sum_{k=0}^\infty \left[ \frac{1}{2}x_{k+1}^\top \matr{Q} x_{k+1} + \frac{1}{2}u_k^\top \matr{R} u_k + x_k^\top \matr{N} u_k \right],  \label{eq:lqr:infinite_obj} \\
    \textrm{s.t. } \quad &\matr{Q} - \matr{N} \matr{R}^{-1} \matr{N}^\top \succ 0, \> \matr{R} > 0 \\
    &x_{k+1} = \matr{A} x_k + \matr{B} u_k \label{eq:lqr:ti_dynamics}
\end{align}

We also consider the finite-horizon case, denoting the horizon by $N^{\mathrm{L}}$. In this case, the $\matr{S}_k$ and $\matr{K}_k$ matrices are time-varying, solved backwards in time using (\ref{eq:lqr:S_tv},~\ref{eq:lqr:K_tv}) from the initial starting point $\matr{S}_{N^{\mathrm{L}}} = \matr{S}_\infty$. The other system matrices can also be time-varying:

\begin{align}
    \matr{S}_{k} &= \matr{Q}_k + \matr{A}_k^\top \matr{S}_{k+1} \matr{A}_k - (\matr{A}_k^\top \matr{S}_{k+1} \matr{B}_k + \matr{R}_k)( \matr{R}_k + \matr{B}_k^\top \matr{S}_{k+1} \matr{B}_k)^{-1} (\matr{B}_k^\top \matr{S}_{k+1} \matr{A}_k + \matr{R}_k^\top) \label{eq:lqr:S_tv} \\
    \matr{K}_k &= -(\matr{R}_k + \matr{B}_k^\top \matr{S}_{k+1} \matr{B}_k)^{-1} (\matr{B}_k^\top \matr{S}_{k+1} \matr{A}_k + \matr{R}_k^\top) \label{eq:lqr:K_tv} \\
    u^{\mathrm{L}}_k(x_k) &= \pi^{\mathrm{L}}_{\theta^{\mathrm{L}}}(x_k) = -\matr{K}_k x_k \label{eq:lqr:control_law_tv}
\end{align}

The finite-horizon \gls{lqr} control problem can then be formally stated as:

\begin{align}
    \min_{x, u} \quad &\sum_{k=0}^{N^{\mathrm{L}}-1} \left[ \frac{1}{2}x_{k+1}^\top \matr{Q} x_{k+1} + \frac{1}{2}u_k^\top \matr{R} u_k + x_k^\top \matr{N} u_k \right],  \label{eq:lqr:finite_obj} \\
    \textrm{s.t. } &\matr{S}_{N^{\mathrm{L}}} = \matr{S}_\infty \\
    \quad &\matr{Q}_k - \matr{N}_k \matr{R}_k^{-1} \matr{N}_k^\top \succ 0, \> \matr{R}_k > 0 \\
    &x_{k+1} = \matr{A}_k x_k + \matr{B}_k u_k \label{eq:lqr:tv_dynamics}
\end{align}

\subsection{Reinforcement Learning}
The system to be optimized in the \gls{rl} framework is formulated as a \gls{mdp}. The \gls{mdp} is defined by a state space $s \in \mathcal{S}$, a set of actions $a \in \mathcal{A}$, a transition probability matrix $\mathcal{T}$ that governs the evolution of states as a function of time and actions, i.e. $s_{t+1} = \mathcal{T}(s_t, a_t)$, a reward function $R(s, a)$ that describes the desirability of the states of the problem, and finally, the discount factor $\gamma \in [0, 1)$ (note the different limits from $\rho$) that describes the relative importance of immediate and future rewards. Note that rewards, $R$, are interchangeable with costs, $C$, through the substitution $R = -C$ (i.e. rewards are negative costs) and changing maximization of the objective to minimization. We will discuss rewards in this section as this is customary in \gls{rl}.

A policy $\pi$ is a function that maps from states to actions, and the goal in \gls{rl} is to find the policy that is optimal in the sense of maximizing the expected sum of discounted rewards, either over an infinite or finite horizon. A policy can be deterministic, which we denote $\pi(s)$, or stochastic, which we denote $\pi(a | s)$ In this paper we study the finite horizon case, and state the objective as:

\begin{align}
    J(\pi) = \mathbb{E}_{s \sim \mathcal{T}(s, \pi(s))}\left[R(s_T) + \sum_{t=0}^{T-1} \gamma^tR(s_t, \pi(s_t))\right] = \mathbb{E}\left[G(\tau)\right] = V^\pi(s_0), \enspace s_0 \in \mathcal{S}_0 \label{eq:rl:obj}
\end{align}

Here, $R(s_T)$ is the terminal reward, $\mathcal{S}_0$ is a distribution of initial states, $G(\tau)$ is the observed return (i.e. sum of discounted rewards) over an episode described by the trajectory $\tau = (s_0, a_1, s_1, \dots, a_{T-1}, s_T)$, $\sim$ signifies that the left hand side is distributed according to the right hand side and the expectation is therefore taken over the state-visitation distribution induced by the transition dynamics and the (possibly stochastic) policy. $V^\pi$ is the value function for the current policy $\pi$.

\subsubsection{Policy Gradient Methods}
Policy gradient algorithms optimizes parameterized policies $\pi_\theta$ directly in the parameter space of the policy, by estimating the gradient of the objective \eqref{eq:rl:obj} and applying a gradient ascent scheme. This is in contrast to other \gls{rl} algorithms that rely on first learning the relative value of the actions available in a given state, and using this information to adjust the action selection probabilities to improve performance. The objective \eqref{eq:rl:obj} depends on the state-visitation distribution, which would require perfect knowledge of the transition dynamics to evaluate. Thus, policy gradients algorithms rely on the policy gradient theorem \eqref{eq:rl:pgt}, which removes this dependence on the state distribution from the gradient \cite{sutton_reinforcement_2018}. The parameters are then updated iteratively according to the gradient estimate and the gradient ascent scheme \eqref{eq:rl:gd}

\begin{align}
    \nabla_\theta J(\theta) &= \mathbb{E}\left[\sum_{t=0}^T \nabla_\theta \log \pi_\theta (a_t | s_t) G(\tau_\theta)\right] \label{eq:rl:pgt} \\
    \theta &= \theta_{\mathrm{old}} + \eta \nabla_\theta J(\theta) \label{eq:rl:gd}
\end{align}

where $\eta$ is the update step size, also called the learning rate. The expectation in \eqref{eq:rl:pgt} can be replaced by sample averages, i.e. to evaluate this gradient, one simply runs the policy on the system to be optimized, and observe the outcomes in terms of returns and state trajectories. Since the update scheme described above is smooth in the parameters, policy gradient methods have good convergence guarantees in theory, but since it is a sampling based approach it suffers from high variance in the gradient estimates in practice \citep{greensmith2004variance,peters_reinforcement_2008}. Thus, advances in these algorithms typically revolve around reducing the variance in these estimates. One important such measure is to alter the return in \eqref{eq:rl:pgt} by subtracting a baseline, e.g. replacing $G(\tau_\theta)$ with the advantage function:

\begin{align}
    A^\pi(s_t, a_t) = R(s_t, a_t) + \gamma V^\pi(s_{t+1}) - V^\pi(s_t) \label{eq:rl:advantage}
\end{align}

The advantage function estimates the value of an action relative to the average value of the actions that the policy would take in that state. Thus, actions that are better than average have positive advantages and vice versa, such that the update procedure above will raise the probability of good actions and decrease the probability of bad actions. This yields faster convergence as opposed to all sampled actions having their probability increased (assuming all rewards are positive) and relying on the fact that better actions with higher rewards are increased in probability faster than bad actions.

\subsection{Proximal Policy Optimization}
\Gls{ppo} \cite{schulman2017proximal} is a policy gradient \gls{rl} algorithm, which is popular due to its data efficiency and simplicity, both in terms of implementation and run-time complexity. The increased data efficiency over other policy gradient algorithms is achieved by modifying the standard policy gradient objective \eqref{eq:rl:obj}, to allow for multiple parameter updates over the same set of data. We include the parameters of the advantage estimator $\hat{A}^{\pi_\theta}$ (and consequently the parameters of the value function estimator $\hat{V}^{\pi_\theta}$) also in the parameter vector $\theta$.

\subsubsection{Trust Region Policy Optimization}
The \gls{ppo} algorithm is inspired by the predecessor \gls{trpo}~\cite{schulman2015trust}, which in a principled way ensures that parameter updates improve upon the objective. This is done by first estimating a region in parameter space where updates are deemed safe in the sense of improving upon the objective, and then identifying the optimal parameter point within this region:

\begin{align}
    \max_\theta \enspace J(\theta) = &\mathbb{E}\left[r(\theta)\hat{A}^{\pi_{\theta_{\mathrm{old}}}}(s, a)\right], \enspace r(\theta) = \frac{\pi_\theta(a | s)}{\pi_{\theta_{\mathrm{old}}}(a | s)}  \\
    s.t.\quad &\mathbb{E}\left[\mathrm{KL}\left(\pi_{\theta_{\mathrm{old}}}(a | s), \pi_\theta(a | s)\right)\right] \leq \delta
\end{align}

Here, $r(\theta)$ is the probability ratio between the policy under two different sets of parameters, $\theta$ and $\theta_{\mathrm{old}}$, the latter of which represents the policy parameters frozen at the start of the parameter update procedure, $\mathrm{KL}$ is the Kullback–Leibler probability divergence measure, and $\delta$ is the maximum allowed divergence. Implementing this update procedure requires second order information about the objective, which is computationally expensive to obtain. 

\subsubsection{The Proximal Policy Optimization Objective}
\gls{ppo} emulates trust region optimization using only first order information, and it is thus considerably more computationally efficient and scalable, while simultaneously empirically demonstrating increased data efficiency. The \gls{ppo} algorithm optimizes a surrogate objective function defined as:

\begin{align}
    J(\theta) &= \mathbb{E}\left[\min\left(r(\theta)\hat{A}^{\pi_{\theta_{\mathrm{old}}}}(s, a), \textrm{clip}\left(r(\theta), 1-\epsilon, 1+\epsilon\right)\hat{A}^{\pi_{\theta_{\mathrm{old}}}}(s, a)\right)\right] \label{eq:ppo:objective}
\end{align}

The probability ratio $r(\theta)$ measures for any given action the ratio of the probability that it would be drawn from the policies in the numerator and denominator. As more parameter updates are performed, the two policies will increasingly differ, and the probability ratio will increasingly deviate from unity. It will be decreasing for actions that are now less likely, and increasing for actions that are more likely under the new parameters. The clip operator ensures that its first argument will be contained in the limits provided as its second and third argument, such that the probability ratio is constrained to the range decided by $\epsilon$, which typically takes on values in the range $0.1 - 0.4$. This ensures that when the advantage of the action is positive the objective value is saturated when the action surpasses $1 + \epsilon$ in increased probability, while when the advantage is negative the objective saturates when the action surpasses $1 - \epsilon$ in decreased probability. Lastly, the minimum operator returns the unclipped objective when the advantage of an action is negative, yet its probability has been increased under the new parameters. The unclipped objective would then make the gradient decrease the probability of this action, correcting the previous update which made the policy worse. This is the mechanism behind \gls{ppo}'s first order approximation of trust region optimization. The gradient of the \gls{ppo} objective \eqref{eq:ppo:objective} is the same as \eqref{eq:rl:pgt}, and is easily obtained with auto-differentiation software.

In practice, the probability ratio $r(\theta)$ is implemented in log space as the difference between the negative action-conditional probability of the policy under the two parameterizations:
\begin{align}
    \log r(\theta) &= \sum_{\tilde{a} \in \mathcal{B}} -\log P_\theta(\tilde{a} | s) - \left(-\log P_{\theta_{\mathrm{old}}}(\tilde{a} | s)\right) \\
    r(\theta) &= \exp(\log r(\theta))
\end{align}

where the notation $\tilde{a}$ signifies an action drawn from the policy's action distribution. The training procedure then involves running the policy in the environment for a number of time steps, generating data on the form $(s_t, \tilde{a}_t, R(s_t, \tilde{a}_t), s_{t+1}, \hat{A}^{\pi_\theta}(s_t, \tilde{a}_t))$ which is stored in a buffer. Then, minibatches $\mathcal{B}$ are sampled from this buffer, the objective \eqref{eq:ppo:objective} and its gradient are evaluated, and the parameters are updated according to \eqref{eq:rl:gd}. This is repeated for the configured number of epochs such that each data point is reused several times, increasing data efficiency.  

\subsubsection{Advantage Function Estimation}

The advantage function is estimated using the \gls{gae} algorithm \cite{schulman2015high}. The advantage is defined in terms of the low bias but high variance information in the sampled rewards $R$, and the high bias but low variance information estimated by the value function $V$. Equation \eqref{eq:rl:advantage} shows the 1-step advantage estimate, which we now denote $\hat{A}_t^{(1)}$, but this can be unrolled further to produce an estimate that contains more information from $R$, and less of the information from $V$. In \gls{gae} this bias-variance tradeoff is summarized as in \eqref{eq:rl:gae} and controlled through the factor $\lambda \in [0, 1]$, where $\lambda = 0$ recovers the 1-step advantage in \eqref{eq:rl:advantage} --- which has the highest bias but lowest variance estimate --- and $\lambda = 1$ corresponds to using all the observed rewards $R$ as an estimate, which yields the lowest bias and the highest variance. The \gls{gae} algorithm \eqref{eq:rl:gae} for $0 < \lambda < 1$ yields a compromise between bias and variance, controlled by $\lambda$, where $H$ is the length of the trajectory collected by the policy:

\iffalse
\begin{align}
    \hat{A}^{(1)}_t &= R(s_t, a_t) + \gamma \hat{V}(s_{t+1}) - \hat{V}(s_t) = \delta^{\hat{V}}_t \\
    \hat{A}^{(2)}_t &= -\hat{V}(s_t) + R(s_t, a_t) + \gamma R(s_{t+1}, a_{t+1}) + \gamma^2 \hat{V}(s_{t+2}) = \delta^{\hat{V}}_t + \delta^{\hat{V}}_{t+1} \\
    \dots& \\
    \hat{A}^{(l)}_t &= \sum_{k=0}^{l-1} \gamma^k \delta^{\hat{V}}_{t+k} \\
    \hat{A}^{\pi_{\theta}}(s_t, a_t) &= (1 - \lambda)(\hat{A}^{(1)}_t + \lambda \hat{A}^{(2)}_t + \lambda^2 \hat{A}^{(3)}_t + \dots) = \sum_{k=0}^T (\gamma \lambda)^k \delta^{\hat{V}^{\pi_{\theta}}}_{t+k} \label{eq:rl:gae}
\end{align}
\fi

\begin{align}
    \hat{A}^{\pi_\theta}(s_t, a_t) &= \delta_t + (\gamma \lambda) \delta_{t+1} + \dots + (\gamma \lambda)^{H-t+1} \delta_{H-1} \label{eq:rl:gae} \\
    \delta_t &= R(s_t, a_t) + \gamma \hat{V}^{\pi_\theta}(s_{t+1}) - \hat{V}^{\pi_\theta}(s_t)
\end{align}
%\todo[inline]{this is for infinite horizon, so how does it fit into the finite horizon case?}

The value function in turn is estimated by a parameterized function approximator $\hat{V}^{\pi_{\theta}}$, that is iteratively improved using fitted value iteration in the manner described by \eqref{eq:val_fn_update}, where $\ell$ corresponds to $R$, $x$ and $\hat{p}$ corresponds to $s$, $u$ corresponds to $a$, and $\rho$ corresponds to $\gamma$.

%One can optionally add a entropy-based objective term that encourages exploration by incentivizing a high entropy in the policy, thus increasing the variability in the actions that are sampled from the policy during training. 

%Maybe talk about global norm constraint and stuff. 
