# Supplementary material for: Optimization of the Model Predictive Control Meta-Parameters Through Reinforcement Learning
Source: arXiv:2111.04146 source file (2021-11-07)
Supplement: Supplementary file 2 [file appendixB.tex]

\section{LQR Weights}
\begin{figure}[hbt!]
    \subfloat[]{\includegraphics[width=0.5\textwidth]{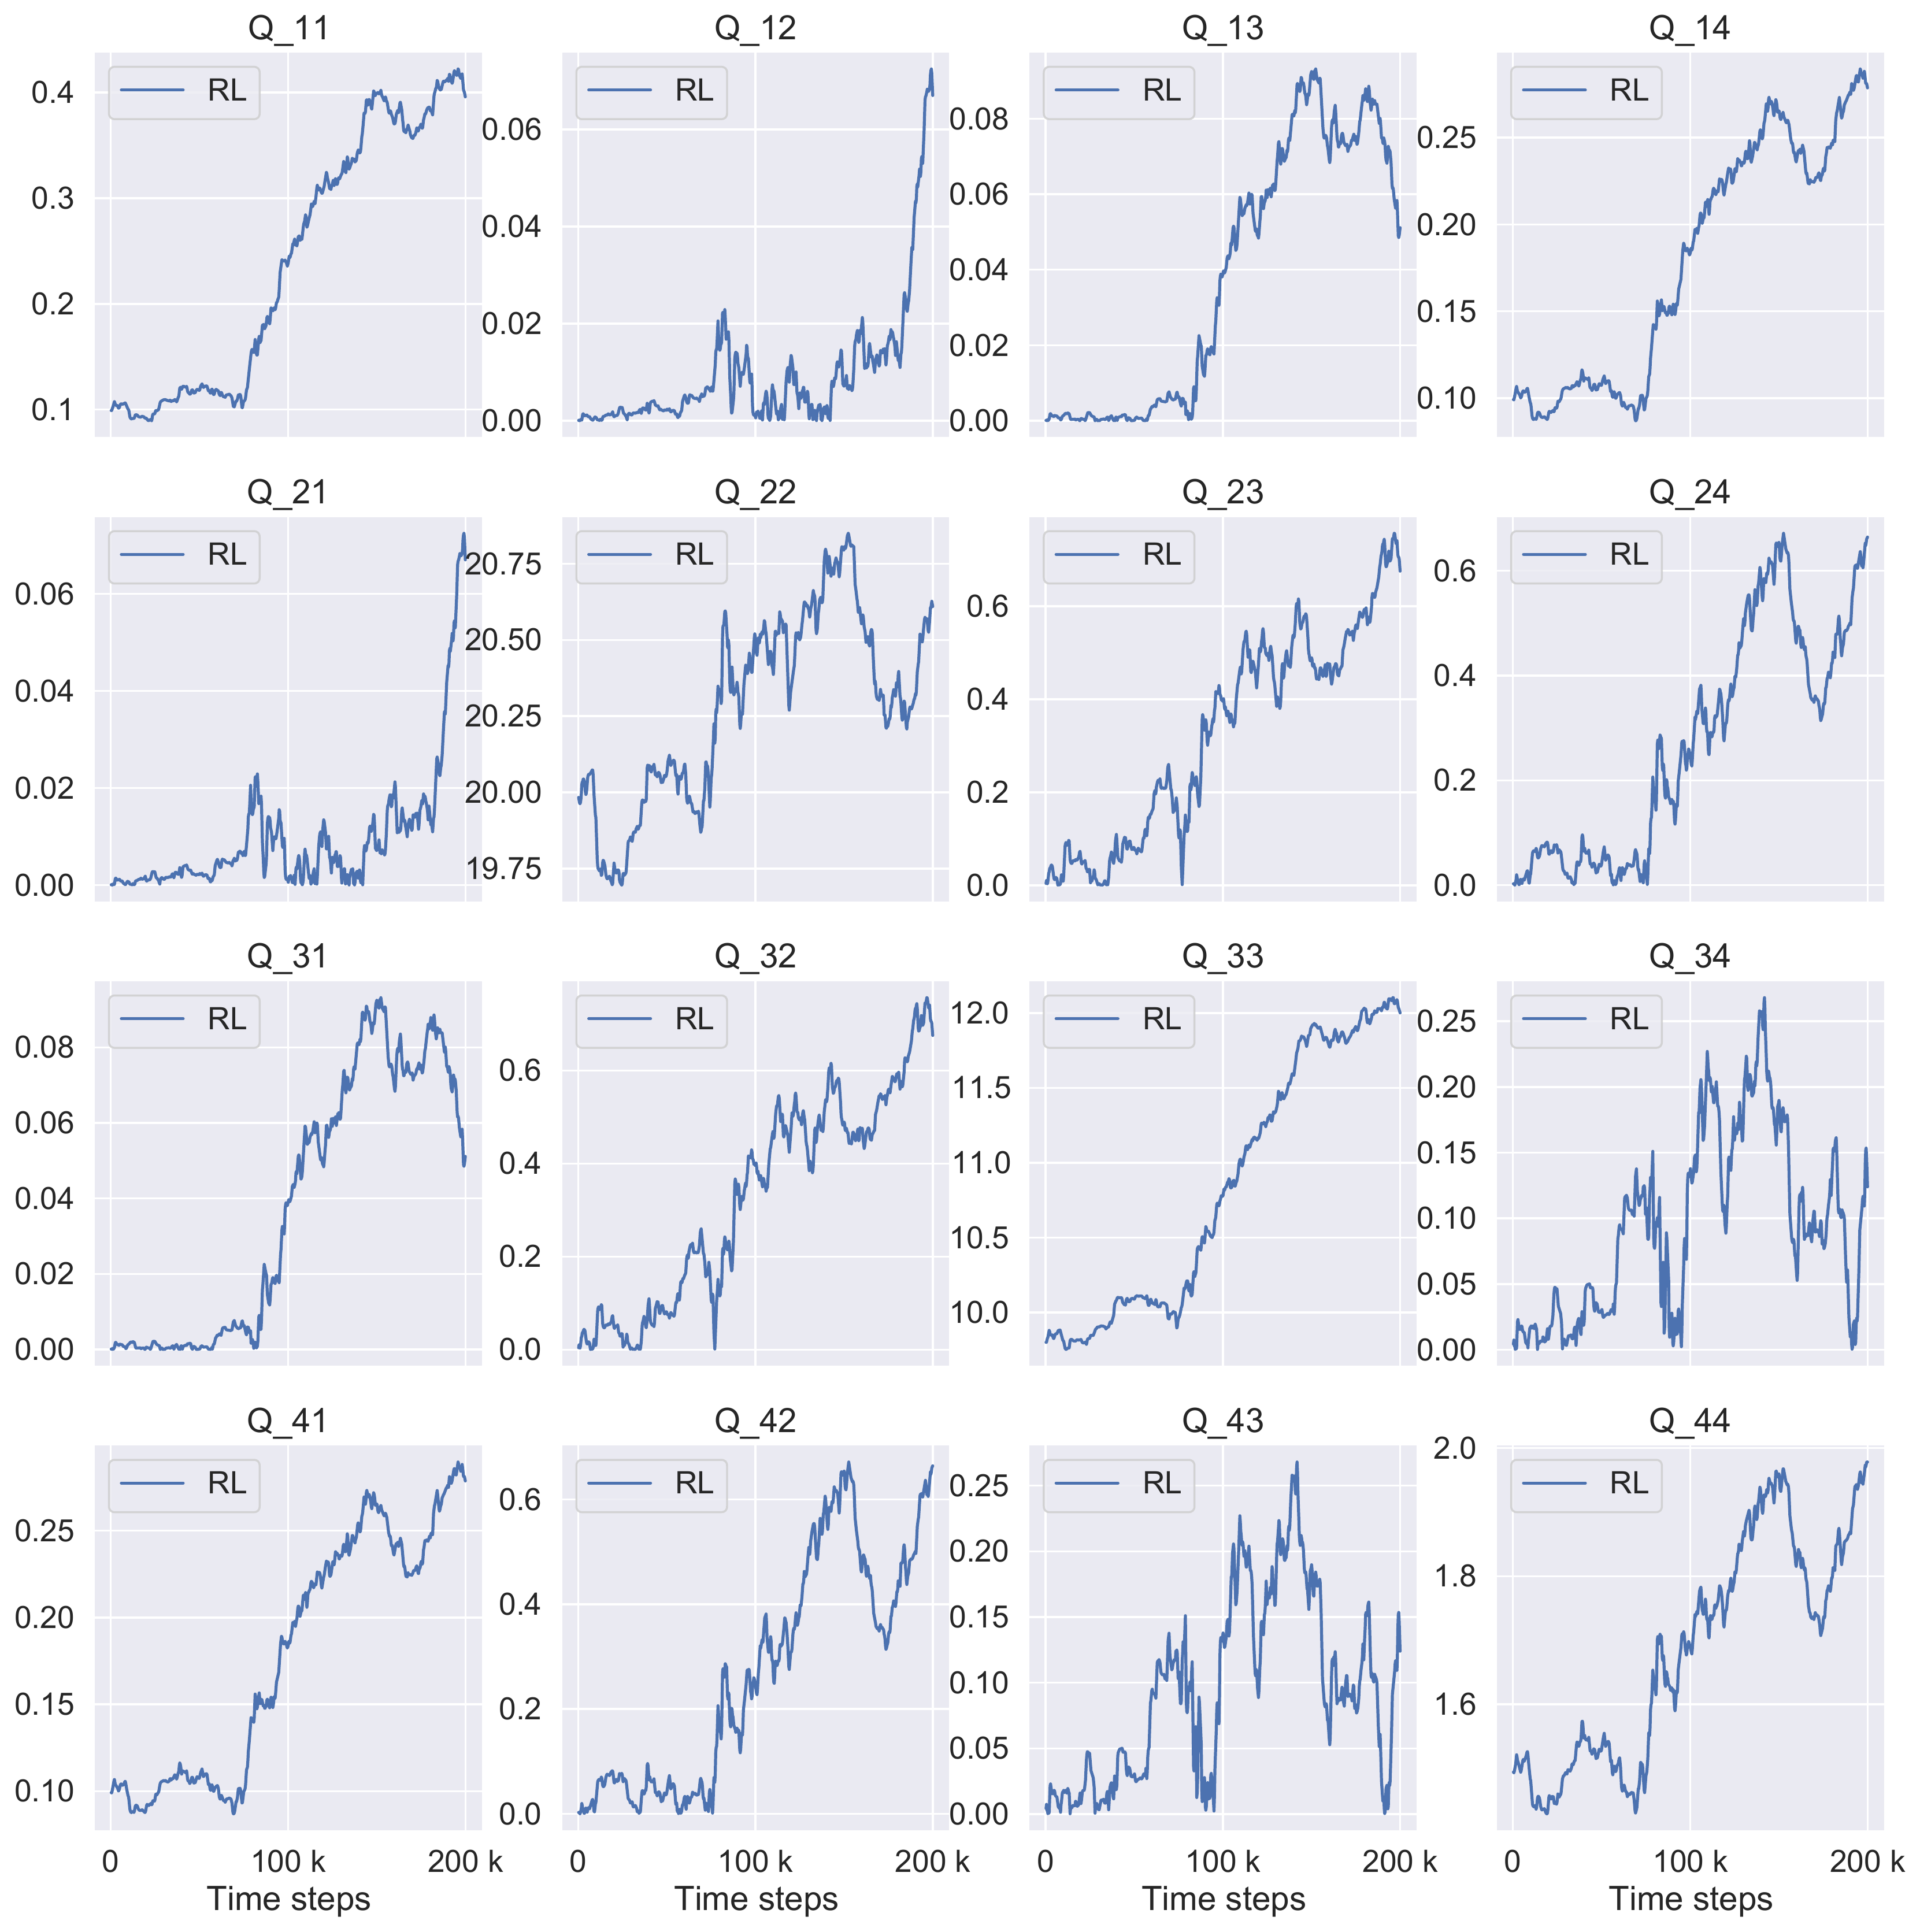}}
    
    \centering
    \subfloat[]{\includegraphics[width=0.125\textwidth]{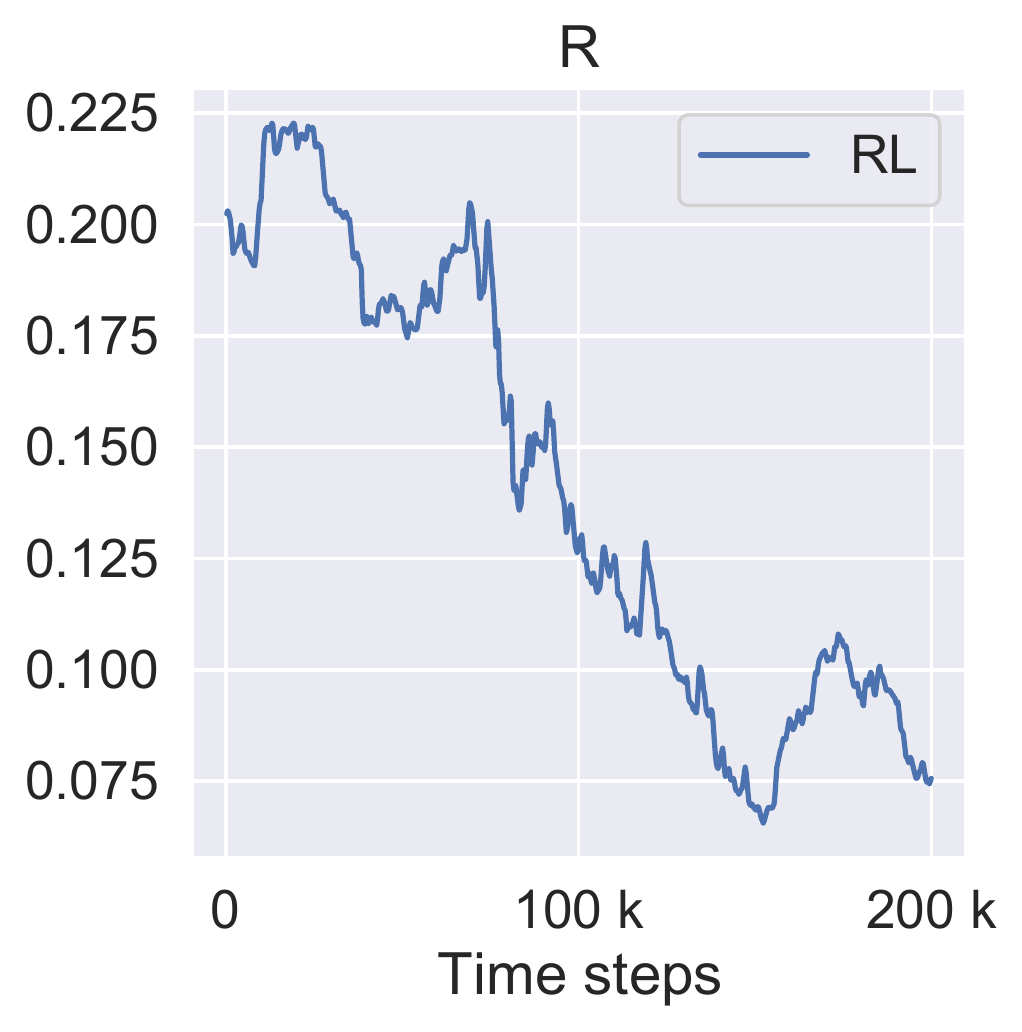}}
    \caption{Evolution of the LQR weights throughout the training of the full control system.}
    \label{fig:appB:lqrweights}
\end{figure}
